# Supplementary material for: Taking Notes Brings Focus? Towards Multi-Turn Multimodal Dialogue Learning
Source: arXiv:2503.07002 source file (2025-03-10)
Supplement: Supplementary file 1 [file prompt_chart_0.pdf]

Please generate a new list based on the provided chart and table data. The main reference should be the chart content, as the table content might contain errors. The format of the new list should be similar to the following example:
[QA_and_CoT]

This list consists of two dictionaries corresponding to two rounds of Q&A. Each question is based on the chart, providing a reasoning process and an answer. The CoT (Chain of Thought) consists of multiple steps with "Ans" representing the answer broken down into steps, and "Query" indicating the key terms in the chart relevant to that step. The final step of CoT provides a complete and concise answer to the question, and the "Query" highlights the key terms in the chart that are relevant to the question.

The Question and CoT answers should be diverse and natural.

**Important**: The second question should refer back to the answer from the first question, meaning that you can't answer the second question unless you know the answer of the first question. The answer of the first question is presented using a pronoun in the second question, and shouldn't appear in the second question.
You only need to output the list in JSON format.

Human:**{Current_QA_and_CoT}**

Please generate a new list based on the provided chart and table data. The main reference should be the chart content, as the table content might contain errors. The format of the new list should be similar to the following example:
[QA_and_CoT]

This list consists of two dictionaries corresponding to two rounds of Q&A. Each question is based on the chart, providing a reasoning process and an answer. The CoT (Chain of Thought) consists of multiple steps with "Ans" representing the answer broken down into steps, and "Query" indicating the key terms in the chart relevant to that step. The final step of CoT provides a complete and concise answer to the question, and the "Query" highlights the key terms in the chart that are relevant to the question.

The Question and CoT answers should be diverse and natural.

**Important**: The second question should refer back to the answer from the first question, meaning that you can't answer the second question unless you know the answer of the first question. The answer of the first question is presented using a pronoun in the second question, and shouldn't appear in the second question.
You only need to output the list in JSON format.

Human:**{Current_QA_and_CoT}**
